# Supplementary material for: In situ tuning of symmetry-breaking induced non-reciprocity in giant-Rashba semiconductor BiTeBr
Source: arXiv:2008.06003 ancillary file (2020-08-17)
Supplement: Supplementary file 1 [file supp.pdf]

# In situ tuning of symmetry-breaking induced non-reciprocity in giant-Rashba semiconductor BiTeBr

Mátyás Kocsis,[†] Oleksandr Zheliuk,[‡] Péter Makk,[†] Endre Tóvári,[†] Péter Kun,[¶] Oleg Evgenevich Tereshchenko,[§,‖,⊥] Konstantin Aleksandrovich Kokh,[§,⊥,#] Takashi Taniguchi,[@] Kenji Watanabe,[△] Justin Ye,[‡] and Szabolcs Csonka[†]

†*Department of Physics, Budapest University of Technology and Economics and MTA-BME Lendület Nanoelectronics Research Group, Budafoki út 8, 1111 Budapest, Hungary*

‡*Zernike Institute for Advanced Materials, University of Groningen, Nijenborgh 4, 9747 AG Groningen, the Netherlands*

¶*Institute of Technical Physics and Materials Science, MFA, Centre for Energy Research, Hungarian Academy of Sciences, P.O. Box 49, 1525 Budapest, Hungary*

§*St. Petersburg State University, 198504, St. Petersburg, Russia.*

‖*A.V. Rzhanov Institute of Semiconductor Physics, 630090, Novosibirsk, Russia.*

⊥*Novosibirsk State University, 630090, Novosibirsk, Russia.*

#*V. S. Sobolev Institute of Geology and Mineralogy, 630090, Novosibirsk, Russia.*

@*International Center for Materials Nanoarchitectonics, National Institute for Materials Science, 1-1 Namiki, Tsukuba 305-0044, Japan*

△*Research Center for Functional Materials, National Institute for Materials Science, 1-1 Namiki, Tsukuba 305-0044, Japan*

Fig. S1.a shows the full IL gating curve of the sample. $V_g$ was ramped first to 2 V, then

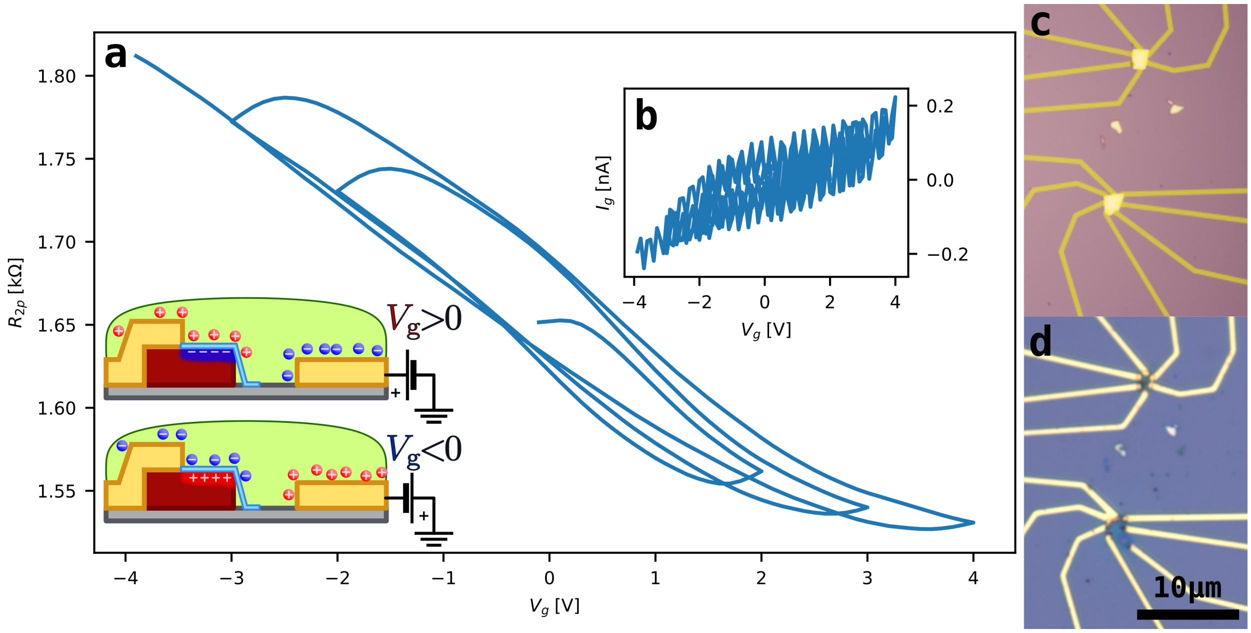


Figure S1: *a)* Full gating curve at 220 K. Hysteretic behaviour is due to the slow movement of the ions. Part of the same curve is shown in Fig. 2. *b)* Gate current as a function of $V_g$. $I_g$ never exceeded 0.3 nA, no chemical reaction takes place between the BiTeBr and the IL. *c)* Optical image of a sample without a hBN protecting layer, before the fabrication of the contacts. Planned contacts are shown in yellow. *d)* Same sample after attempting IL gating. The BiTeBr flakes that were contacted are completely dissolved, while the smaller, uncontacted crystals are only moved by the application and washing off of the IL.

with each sweep successively increased to 4 V, which is still well within the electrochemical window of DEME-TFSI. The gate current was continually monitored, and increased with increasing $V_g$, but never exceeded 0.3 nA, as is shown in Fig. S1.b.

When IL gating was attempted on uncovered BiTeBr samples shown in Fig. S1.c, the samples decomposed, while smaller BiTeBr that were not contacted only shifted slightly by the application and washing off of the IL.

Due to the positioning of the contacts on the sample, Hall measurements could only be carried out in non-optimal geometries, as shown in the insets of Fig. S2.a. This meant that instead of measuring $R_{xy}$, the measured values are a mixture of $R_{xx}$ and $R_{xy}$. To distinguish the two components, we anti-symmetrized the signal, yielding only the $R_{xy}$ component, which was used to calculate the electron density. We note that a small error may remain due to the inhomogenity of the current density.

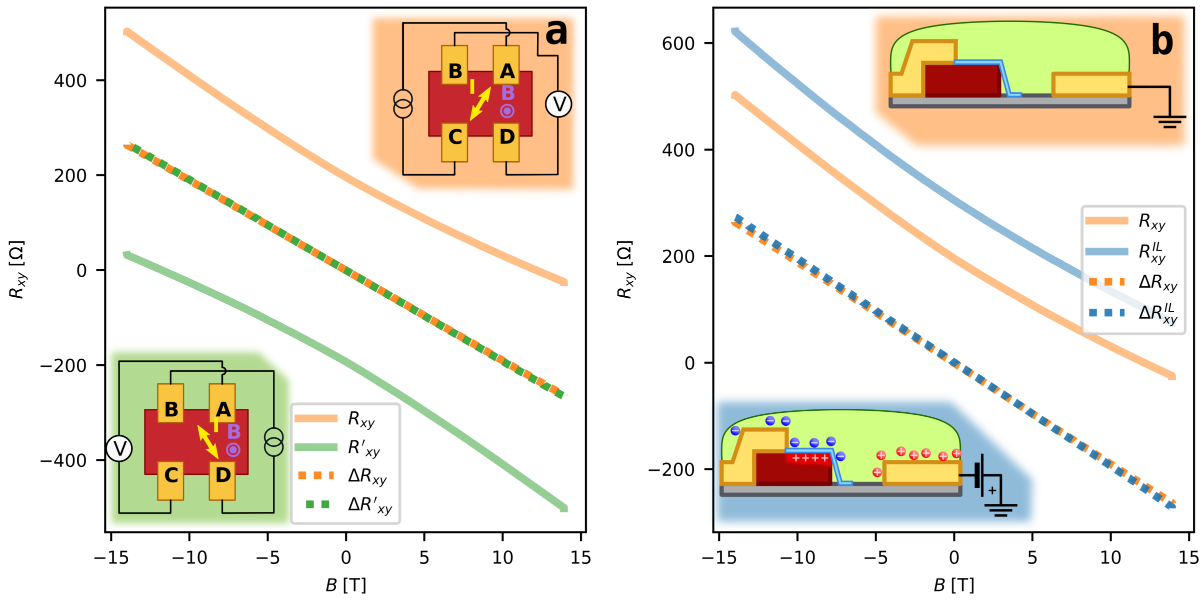


Figure S2: *a)* Hall measurements before the IL was applied. $R_{xy}$ (solid lines) and its anti-symmetrized component $\Delta R_{xy}$ (dotted lines) as a function of the out-of-plane magnetic field. The anti-symmetrization is necessary, as the non-optimal geometry of the sample leads to the mixing of the $R_{xx}$ and $R_{xy}$ components. Insets show the respective geometries for the two measurements. They both yield the same value for $n$. *b)* Hall measurements without the IL applied (orange) and $V_{\mathrm{g}} = -4\,\mathrm{V}$ (blue). The orange curve is the same as in panel a. The calculated electron densities are shown in Fig. 4.

As mentioned in the main text,

$$\Delta R^{2\omega} \propto B \times I\gamma'. \tag{S1}$$

By measuring $\Delta R^{2\omega}$ as a function of $B$ or $I$ we can calculate $\gamma'$. While the main article dealt exclusively with the $B$ dependence, here we explore how the non-reciprocity depends on the applied current. Fig. S3.a shows $\Delta R^{2\omega}$ as a function of $B$, at different applied currents ($5\,\mu\mathrm{A}$ to $80\,\mu\mathrm{A}$, see panel b). As $\gamma'$ is related to the slope of the curves, we would expect the low current measurements to yield significantly shallower slopes, but this is not the case. To understand the situation better, we plotted the maxima of $\Delta R^{2\omega}$ from panel a as a function of $I$ in Fig. S3.b. While the data could be fit with a linear function, it has a significant offset, and does not cross the origin as equation (S1) would suggest. Since $\gamma'$ is calculated

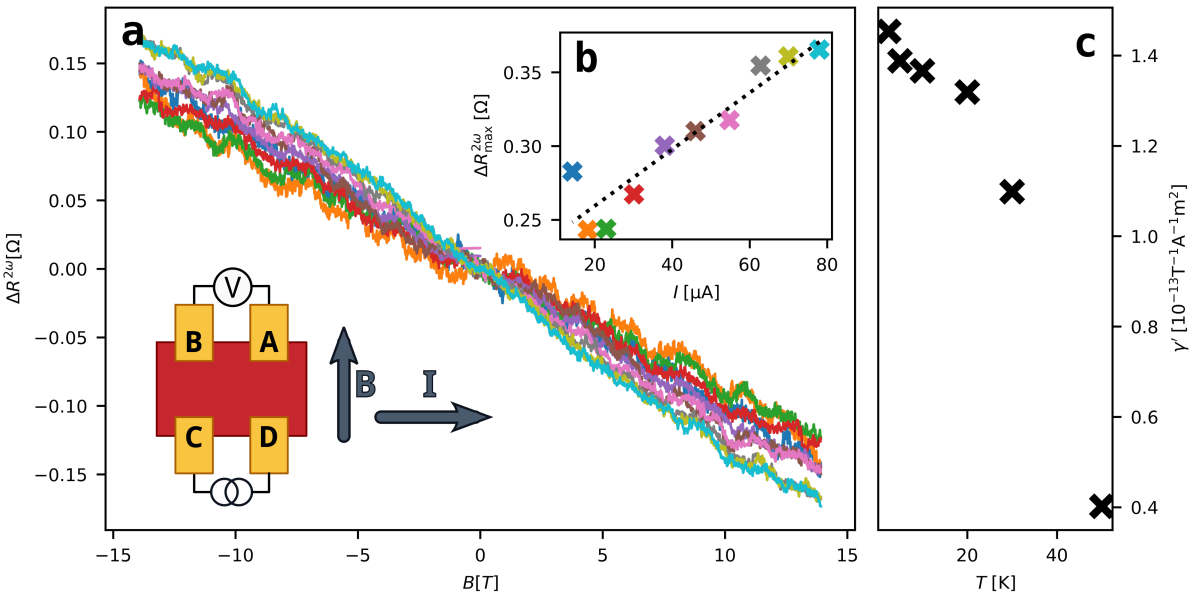


Figure S3: All measurements were carried out at 2.5 K before applying the IL. *a)* $\Delta R^{2\omega}$ as a function of the magnetic field, for different applied current amplitudes. The non-reciprocity is expected to scale with the current as Equation (S1) shows, the measured change is quite small however. *b)* $\Delta R^{2\omega}_{\mathbf{B=15T}}$ acquired from linear fits as a function of the applied current. While the trend is linear, it does not cross the axes at the origin, it has a 0.22 Ω offset. *c)* Temperature dependence of $\gamma'$ follow the same trend as results in Ref. 1.

by dividing $\Delta R^{2\omega}$ by $I$, this offset becomes more significant at small $I$. To avoid the effects of this offset all other measurements were carried out at 80 µA to 100 µA, as higher currents would have likely damaged the device. The source of this offset is not known.

The temperature dependence of $\gamma'$ is shown in Fig. S3.c, it follows the same trend as the theory presented in Ref. 1.

The geometry of each sample was measured using AFM. An AFM image of the sample discussed in the main article is shown in the inset of Fig. S4. The higher (white, blue) BiTeBr flakes are covered with the few nm thin hBN flake (pink). To measure the height of the BiTeBr flake, the height distribution in the region outlined in red was measured. As both the substrate and the BiTeBr flake are covered by the hBN, the origin was shifted to the height of the hBN layer. From this the height of the flake is $(39.0 \pm 0.6)$ nm.

The flakes obtained by exfoliation from the same bulk crystals could be classified into

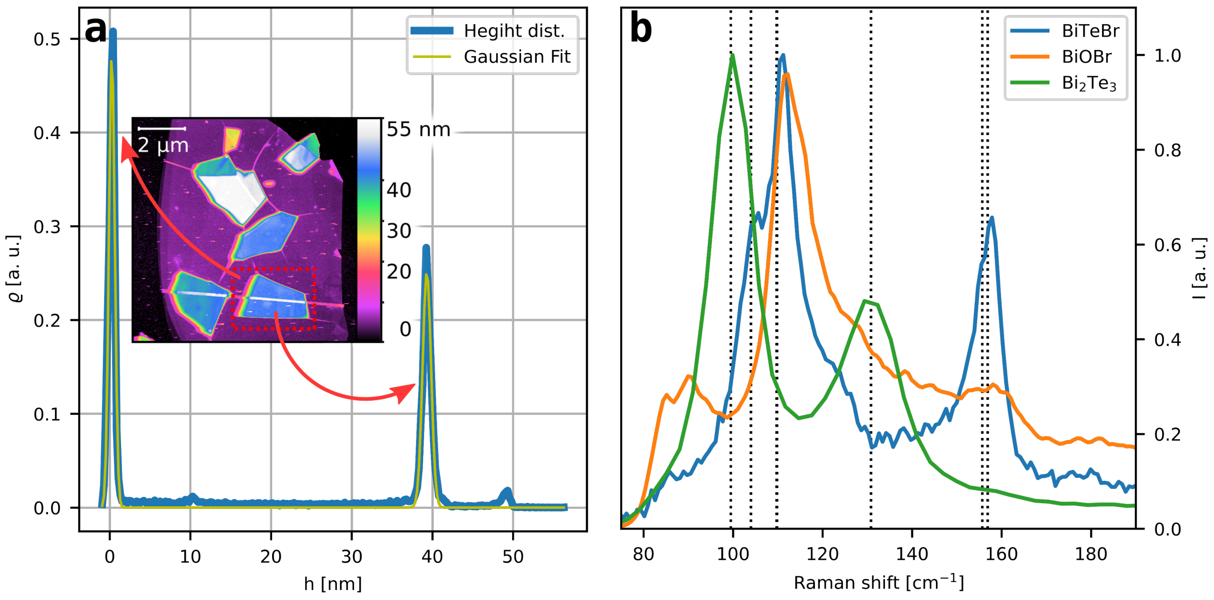


Figure S4: *a)* AFM image of the sample discussed in the main article. The height of the sample was measured by fitting the height distribution of the area highlighted with a dashed red rectangle. The height was measured from the top of the hBN flake to the top of the hBN+BiTeBr stack. *b)* Raman spectra of different flakes obtained from the same bulk crystals during exfoliation. The grey dashed lines mark the peaks calculated using DFT in Ref. 2. The blue spectrum shows good agreement with the results of Ref. 2 and Ref. 3, and EDS measurements confirmed the presence of Bi, Te, and Br. The green spectrum shows good agreement with the results of Ref. 4 (where it is identified as BiTeBr) and Ref. 5, 6 (where it is identified as $Bi_2Te_3$), while EDS measurements show a lack of Br. The flakes showing the orange spectrum are insulating, and not opaque, displaying different colours based on their thickness. The spectrum aligns with that in Ref. 7 where it is identified as BiOBr. EDS measurements confirm a lack of Te, while the excess O could not be clearly seen due to the background signal of the SiO substrate.

three categories. The first is made up of white flakes 35 nm and thicker, which are conductive and show the non-reciprocal phenomena discussed in the main article. This has been confirmed on other flakes, not discussed in this article. Flakes in the second class can be thinner, from 5 nm up to more than 100 nm, are not opaque and colourful, and insulating. The third are white and thick, resembling the first class, but do not show the non-reciprocal behaviour.

To understand the cause of the differences, we carried out Raman and EDS measurements on all classes of flakes. Fig. S4.b shows the three distinct types of Raman spectra obtained.

The first class showed the expected[2,3] Raman spectra, and the EDS confirmed the presence of Bi, Te, and Br. The second class showed the Raman spectra of BiOBr,[7] and the EDS confirmed the lack of Te. The spectra of the third class resembles that of $Bi_2Te_3$,[5,6] EDS measurements confirmed the lack of Br.

This means that Raman characterization is crucial for all heterostructures.

# References


(1) Ideue, T.; Hamamoto, K.; Koshikawa, S.; Ezawa, M.; Shimizu, S.; Kaneko, Y.; Tokura, Y.; Nagaosa, N.; Iwasa, Y. Bulk rectification effect in a polar semiconductor. *Nature Physics* **2017**, *13*, 578–583.

(2) Sans, J. A.; Manjón, F. J.; Pereira, A. L. J.; Vilaplana, R.; Gomis, O.; Segura, A.; Muñoz, A.; Rodríguez-Hernández, P.; Popescu, C.; Drasar, C.; Ruleova, P. Structural, vibrational, and electrical study of compressed BiTeBr. *Physical Review B* **2016**, *93*.

(3) Akrap, A.; Teyssier, J.; Magrez, A.; Bugnon, P.; Berger, H.; Kuzmenko, A. B.; van der Marel, D. Optical properties of BiTeBr and BiTeCl. *Physical Review B* **2014**, *90*.

(4) Sklyadneva, I. Y.; Heid, R.; Bohnen, K.-P.; Chis, V.; Volodin, V. A.; Kokh, K. A.; Tereshchenko, O. E.; Echenique, P. M.; Chulkov, E. V. Lattice dynamics of bismuth tellurohalides. *Phys. Rev. B* **2012**, *86*, 094302.

(5) Shahil, K. M. F.; Hossain, M. Z.; Goyal, V.; Balandin, A. A. Micro-Raman spectroscopy of mechanically exfoliated few-quintuple layers of Bi $_2$ Te $_3$ , Bi $_2$ Se $_3$ , and Sb $_2$ Te $_3$ materials. *Journal of Applied Physics* **2012**, *111*, 054305.

(6) Goncalves, L. M.; Couto, C.; Alpuim, P.; Rolo, A. G.; Völklein, F.; Correia, J. H. Optimization of thermoelectric properties on Bi2Te3 thin films deposited by thermal co-evaporation. *Thin Solid Films* **2010**, *518*, 2816–2821.

(7) Davies, J. E. D. Solid state vibrational spectroscopy—III[1] The infrared and raman spectra of the bismuth(III) oxide halides. *Journal of Inorganic and Nuclear Chemistry* **1973**, *35*, 1531–1534.
